# Supplementary material for: Dynamic Boundary Time Warping for Sub-sequence Matching with Few Examples
Source: arXiv:2010.14464 source file (2024-09-01)
Supplement: Supplementary file 1 [file appendix.tex]

% put an appendix here if needed (after bibliography)
